# Supplementary material for: Hyperbolic Secant representation of the logistic function: Application to probabilistic Multiple Instance Learning for CT intracranial hemorrhage detection
Source: arXiv:2403.14829 source file (2024-03-21)
Supplement: Supplementary file 1 [file appendix_equivalence.tex]

\section{Equivalence for the general logistic model}\label{appendix:equivalence}

%\subsection{Equivalence}\label{subsection:logistic_equivalence}

We generalize the equivalence we observed for GPs to a general setting. For this purpose, we consider the \emph{general logistic model}. 

\begin{definition}
    The general logistic model is
        \begin{equation}
        \p(\bu, \bff, \by, \bT) = \p(\bu) \p(\bff \mid \bu) \p(\by \mid \bff) \p(\bT \mid \by),
    \end{equation}
    where $\bff = \left[ f_1, \ldots, f_N \right]^\top$, $\p(\by \mid \bff) = \prod_n \p(y_n \mid f_n)$ and $\p(y_n \mid f_n) = \operatorname{Ber}(y_n \mid \logit(f_n))$. The set of all observed variables is denoted by $\bE$ and the rest by $\bA$.
\end{definition}
Note that we make no assumptions about the distributions that $\bu$, $\bff$ and $\bT$ follow. That is, $\bu$, $\bff$ and $\bT$ need not to satisfy Eq. \eqref{eq:u_prob}, \eqref{eq:f_prob} and \eqref{eq:bag_prob}. Also, this setting contemplates both the classic supervised and MIL scenarios. In the classic supervised setting, $\bA = \left\{ \bu, \bff\right\}$ and $\bE = \left\{ \by, \bT\right\}$, where $\bT = \left[ \widetilde{y}_1, \ldots, \widetilde{y}_N\right]^\top$ is any variable such that $\p(\widetilde{y}_n \mid y_n) = 1$ if $\widetilde{y}_n = y_n$ and $0$ otherwise. In the MIL setting, $\bA = \left\{ \bu, \bff, \by \right\}$ and $\bE = \left\{ \bT\right\}$, where  $\bT = \left[ T_1, \ldots, T_B\right]^\top$ are the observed bag labels, while the instance labels $\by$ remain unobserved. 

Our ultimate goal is to approximate the posterior $\p(\bA \mid \bE)$ by a variational distribution $\q(\bA)$, which is chosen by maximizing the following ELBO:
\begin{equation}
    \ELBO(\q(\bA)) = \Ebb_{\q(\bA)} \left[ \log \frac{\p(\bu, \bff, \by, \bT)}{\q(\bA)}\right].
\end{equation}
Since this objective is intractable due to the presence of the logistic observation model, we must consider either the SG or the GSM representation. 

\noindent\textbf{Using the SG representation}. In this case, we maximize a lower bound on the true ELBO, 
\begin{equation}\label{eq:ELBO_SG}
    \ELBO \geq \ELBO_{\mathrm{SG}}(\q(\bA), \bxi) = \Ebb_{\q(\bA)} \left[ \log \frac{\J(\bu, \bff, \by, \bxi, \bT)}{\q(\bA)}\right],
\end{equation}
where 
\begin{equation}
    \J(\bu, \bff, \by, \bT) = \p(\bu) \p(\bff \mid \bu) \J(\by \mid \bff, \bxi) \p(\bT \mid \by),
\end{equation}
where $\J(\by \mid \bff, \bxi) = \prod_n \J(y_n \mid f_n, \xi_n)$ and $\J(y_n \mid f_n, \xi_n)$ is defined as in Eq. \eqref{eq:J_y_f_xi}. 
The corresponding variational update equation for $\q(\bA)$ becomes
\begin{align}\label{eq:q_SG}
    \log \q_{\mathrm{SG}}(\bA) = & \log \left( \p(\bu) \p(\bff \mid \bu) \p(\bT \mid \by)\right) + \\
    & + \left( \by - 2^{-1} \right)^\top \bff - 2^{-1} \bff^\top \bLambda \bff + \const,
\end{align}
where $\bLambda = \diag \left( 2\lambda(\xi_1), \ldots, 2\lambda(\xi_N)\right)$ and $\const$ is a term that does not depend on $\bA$. 

\noindent\textbf{Using the GSM representation}. Instead, if we use the GSM representation, we consider the augmented joint probability
\begin{equation}
    \p(\bu, \bff, \by, \bomega, \bT) = \p(\bu) \p(\bff \mid \bu) \p(\by, \bomega \mid \bff) \p(\bT \mid \by),
\end{equation}
where $\p(\by, \bomega \mid \bff) = \prod_n \p(y_n, \omega_n \mid f_n)$ and $\p(y_n, \omega_n, \mid f_n)$ is defined as in Eq. \eqref{eq:p_y_omega_gsm}. The ELBO to be maximized in the GSM setting is 
\begin{equation}\label{eq:ELBO_GSM}
    \ELBO_{\mathrm{GSM}}(\q(\bA), \q(\bomega)) = \Ebb_{\q(\bA)\q(\bomega)} \left[ \log \frac{\p(\bu, \bff, \by, \bomega, \bT)}{\q(\bA)\q(\bomega)}\right]. 
\end{equation}
The GSM variational update equation of $\q(\bA)$ becomes
\begin{align}\label{eq:q_GSM}
    \log \q_{\mathrm{GSM}}(\bA) = & \log \left( \p(\bu) \p(\bff \mid \bu) \p(\bT \mid \by)\right) + \\
    & + \left( \by - 2^{-1}\mathbf{1} \right)^\top \bff - 2^{-1} \bff^\top \bTheta \bff + \const,
\end{align}
where $\bTheta = \diag \left( \Ebb_{\q(\omega_1)}\left[ \omega_1 \right], \ldots, \Ebb_{\q(\omega_N)}\left[ \omega_N \right]\right)$ and $\const$ is a term that does not depend on $\bA$. Note that only the expectation of the approximated posterior $\q(\omega_n)$ is needed to compute $\q_{\mathrm{GSM}}(\bA)$. We will take advantage of this later. 

As in VGPMIL, Eq. \eqref{eq:q_SG} and \eqref{eq:q_GSM} differ only in the matrices $\bLambda$ and $\bTheta$, which become equal once $\bxi$ and $\q(\bomega)$ are set to their optimal values. These are given by the following proposition. 

\begin{proposition}\label{prop:optimal_xi_omega}
%[][normal,no link to proof, text proof={Proof of Proposition \string\ref{thm:prAtEnd\pratendcountercurrent}}]
    Fixed $\q(\bA)$, 
    \begin{enumerate}
        \item The optimal value of $\bxi = \left[ \xi_1, \ldots, \xi_N\right]^\top$ in Eq. \eqref{eq:ELBO_SG} is given by 
        \begin{equation}\label{eq:xi_optimal}
            \xi_n^2 = \Ebb_{\q(\bA)} \left[ f_n^2 \right].
        \end{equation}
        \item The optimal value of $\q(\bomega) = \prod_n \q(\omega_n)$ in Eq. \eqref{eq:ELBO_GSM} is given by
        \begin{equation}\label{eq:omega_optimal}
            \q(\omega_n) = \phi(\omega_n \mid f_n = \xi_n) = \PG(\omega_n \mid 1, \xi_n),
        \end{equation}
        where $\xi_n^2 = \Ebb_{\q(\bA)} \left[ f_n^2 \right]$. 
    \end{enumerate}    
\end{proposition}
\begin{proof}
    See Subsection \ref{subsection:proofs_equivalence}
\end{proof}

We can use the same argument from Subsection \ref{subsection:pg4gpmil_equivalence} to conclude that the SG and GSM representations lead to the same variational updates. This is the same behavior that we observed when we proposed PG-VGPMIL. To explain why this happens, we explore the relationship that exists between $\ELBO_{\mathrm{SG}}$ and $\ELBO_{\mathrm{GSM}}$. The following result summarizes our findings. 

\begin{propositionE}%[][normal,no link to proof, text proof={Proof of Proposition \string\ref{thm:prAtEnd\pratendcountercurrent}}]
\label{prop:elbo_equality}
    Let $\xi_n \in \left]0, +\infty \right[$ and $\q(\omega_n) = \PG(\omega_n \mid 1, \xi_n)$. Then, 
    \begin{equation}
        \ELBO_{\mathrm{SG}}(\q(\bA), \bxi) = \ELBO_{\mathrm{GSM}}(\q(\bA), \q(\bomega)).
    \end{equation}
\end{propositionE}
\begin{proof}
    See Subsection \ref{subsection:proofs_equivalence}.
\end{proof}

This means that, when we restrict $\q(\omega_n)$ to belong to a particular family of densities, the Pólya-Gamma family, both optimization objectives become equal. This family appears in Proposition \ref{prop:optimal_xi_omega} as the optimal variational distribution of $\omega_n$. Therefore, both approaches lead to identical variational posterior distributions because, in fact, the underlying optimization objective is the same (once $\xi_n$ and $\q(\omega_n)$ are defined to take their optimal values). 

\subsection{Proofs}\label{subsection:proofs_equivalence}
\begin{proof}[Proof of Proposition \ref{prop:optimal_xi_omega}]

    Before proceeding with this proof, we need to state and prove two intermediate results.
    
    \begin{lemma}\label{lemma:phi_posterior}
    For any $\omega \in \left]0, + \infty\right[$ and $x \in \R$,
    \begin{equation}
        \phi(\omega \mid x) = \PG \left( \omega \mid 1, x\right).
    \end{equation}
    \end{lemma}
    \begin{proof}%[Proof of Lemma \ref{lemma:phi_posterior}]
    We have     
    \begin{gather}
        \phi(\omega \mid x) = \phi(x)^{-1} \phi(x \mid \omega) \phi_\omega(\omega),\\
        \phi(x) = \left( 2 \pi \cosh(x/2) \right)^{-1}, \\
        \phi(x \mid \omega) \phi_\omega(\omega) = (2\pi)^{-1} \exp\left( - x^2 \omega / 2 \right) \PG(\omega \mid 1, 0).
    \end{gather}
    Then, we use $\PG \left( \omega \mid 1, c\right) = \cosh\left( c/2 \right) \exp\left( - c^2 \omega / 2 \right) \PG(\omega \mid 1, 0)$ from \cite{polson2013bayesian} to conclude the proof.
    \end{proof}
    
    \begin{lemma}\label{lemma:optimal_xi_function}
    Let $a \in \mathbb{R}$ and $b \in \R$. We consider the function defined for each $x \in \left]0, +\infty\right[$ by 
    \begin{equation}
        h(x) = \lambda(x)\left( x^2 - a^2 \right) + \log \phi(x) + b.
    \end{equation}
    Then $h$ reaches an absolute maximum at $x = a$. 
    \end{lemma}
    \begin{proof}%[Proof of Lemma \ref{lemma:optimal_xi_function}]
    The function $h$ is differentiable with 
    \begin{equation}
        h'(x) = \lambda'(x) \left( x^2 - a^2 \right),
    \end{equation}
    for each $x \in \R$. Since $\lambda$ is strictly decreasing in $\left]0, +\infty\right[$, the function $h'$ only becomes zero at $x=a$ and this is an absolute maximum.
    \end{proof}

    Now, we can proceed with the proof of Proposition \ref{prop:optimal_xi_omega}. We begin by proving the first assertion. We have
    \begin{align}
        \ELBO_{\mathrm{SG}}(\q(\bA), \bxi) & = \sum_n \Ebb_{\q(\bA)} \left[   \log \J(y_n \mid f_n, \xi_n^*) \right] + \const = \\
        & = \sum_n \left\{ \lambda(\xi_n)\left(\xi_n^2 - \Ebb_{\q(\bA)} \left[f_n^2\right] \right) + \log \phi(\xi_n) \right\} + \const,
    \end{align}
    where $\const$ is a sum of terms that do not depend on $\bxi$. For each summand, we can apply Lemma \ref{lemma:optimal_xi_function} to obtain the desired result. 
    For the second assertion, observe that we are employing the mean-field variational approximation, so we can obtain the solution to the factor $\q(\omega_n)$ using \cite[Equation (10.9)]{bishop2006pattern}, 
    \begin{align}
        \log \q(\omega_n) & = \Ebb_{\q(\bA)} \left[ \log \p(y_n, \omega_n \mid f_n)\right] + \const = \\
        & = \Ebb_{\q(\bA)} \left[ \log \phi(f_n \mid \omega_n) \right] + \log \phi_\omega(\omega_n) + \const.
    \end{align}
    A simple computation reveals that $\Ebb_{\q(\bA)} \left[ \log \phi(f_n \mid \omega_n) \right] = \log \mathcal{N}\left( \xi_n \mid 0, \omega_n \right) = \log \phi(f_n = \xi_n \mid \omega_n)$. Therefore, 
    \begin{align}
        \q(\omega_n) = \frac{\phi(f_n = \xi_n \mid \omega_n) \phi_\omega(\omega_n)}{\phi(f_n = \xi_n)} = \phi(\omega_n \mid f_n = \xi_n).
    \end{align}    
    Finally, we apply Lemma \ref{lemma:phi_posterior} to obtain the desired result. 
\end{proof}

\begin{proof}[Proof of Proposition \ref{prop:elbo_equality}]

The first step is to establish a connection between the Jaakkola bound and the Pólya-Gamma distribution, which is given by the following result. 

    \begin{proposition}\label{prop:sg_gsm_relation}
        Let $\xi_n \in \left]0, +\infty \right[$. Then, 
        \begin{equation}
            \log \J(y_n \mid f_n, \xi_n) = \Ebb_{\PG(\omega_n \mid 1, \xi_n)} \left[ \log \frac{\p(y_n, \omega_n \mid f_n)}{\PG(\omega_n \mid 1, \xi_n)} \right]
        \end{equation}
    \end{proposition}
    \begin{proof}
        We write $\p(\omega_n) = \PG\left( \omega_n \mid 1,0 \right)$ and $\q(\omega_n) = \PG(\omega_n \mid 1, \xi_n)$. Remember that $\Ebb_{\q(\omega_n)} \left[ \omega_n \right] = \tanh(\xi_n/2)/(2\xi_n) = 2\lambda(\xi_n)$. Using this and the expression of the Kullback-Leibler divergence between two Pólya-Gamma distributions (see \cite{wenzel2019efficient} for the details on the derivation) we obtain
        \begin{align}
            \log \J(y_n \mid f_n, \xi_n) = &  \log \pi + (y_n-1/2)f_n -\lambda(\xi_n) f_n^2 + \\
            & + \log \phi(\xi_n) + \lambda(\xi_n)\xi_n^2 = \\
            = & - \log 2 + (y_n-1/2)f_n - 2^{-1} \Ebb_{\q(\omega_n)} \left[ \omega_n \right] f_n^2 + \\
            & - \log \cosh (\xi_n/2) + (\xi_n/4) \tanh\left(\xi_n/2\right) = \\ 
            = &- \log 2 + (y_n-1/2)f_n - 2^{-1} \Ebb_{\q(\omega_n)} \left[ \omega_n \right] f_n^2 + \\
            & - \D_{\KL}\left[ \q(\omega_n) , \p(\omega_n) \right] = \\
            = &  \Ebb_{\q(\omega_n)} \left[ \log \frac{\p(y_n, \omega_n \mid f_n)}{\q(\omega_n)} \right].
        \end{align}
    \end{proof}

    Next, observe that 
    \begin{align}
        \ELBO_{\mathrm{SG}}(\q(\bA), \bxi) & = \Ebb_{\q(\bA)} \left[ \log \frac{\p(\bu) \p(\bff \mid \bu) \p(\bT \mid \by)}{\q(\bA)}\right] + \\
        & + \Ebb_{\q(\bA)} \left[ \sum_n  \log \J(y_n \mid f_n, \xi_n) \right],
    \end{align}
    and
    \begin{align}
        \ELBO_{\mathrm{GSM}}(\q(\bA), \q(\bomega)) & = \Ebb_{\q(\bA)} \left[ \log \frac{\p(\bu) \p(\bff \mid \bu) \p(\bT \mid \by)}{\q(\bA)}\right] + \\
        & + \Ebb_{\q(\bA)} \left[ \sum_n \Ebb_{\q(\omega_n)} \left[\log \frac{\p(y_n, \omega_n \mid f_n)}{\q(\omega_n)} \right] \right]. 
    \end{align}
    Finally, apply Proposition \ref{prop:sg_gsm_relation} to obtain the desired equality.    
\end{proof}
