# Supplementary material for: Hyperbolic Secant representation of the logistic function: Application to probabilistic Multiple Instance Learning for CT intracranial hemorrhage detection
Source: arXiv:2403.14829 source file (2024-03-21)
Supplement: Supplementary file 2 [file appendix_representations.tex]

\section{Proofs of Proposition \ref{prop:phi_sg} and Proposition \ref{prop:phi_gsm}}\label{appendix:proofs}

\begin{proof}[Proof of Proposition \ref{prop:phi_sg}]
    Equivalently, we show that $s \mapsto g_\phi'(s)/s = \tanh(s/2)/(2s)$ is decreasing in $\left]0, +\infty\right[$ by taking its derivative and studying the monotonicity. Write, for $s \in \left]0, +\infty\right[$,
    \begin{equation}
        h(s) = \frac{\tanh(s/2)}{2s} = \frac{\exp(s/2) - \exp(-s/2)}{2s(\exp(s/2) + \exp(-s/2))}.
    \end{equation}
    Then, 
    \begin{equation}
        h'(s) = \frac{2s + \exp(-s) - \exp(s)}{4s^2(\exp(s/2) + \exp(-s/2))^2}.
    \end{equation}
    Because $4s^2(\exp(s/2) + \exp(-s/2))^2 > 0$, the proof will be concluded when we show $r(s) = 2s + \exp(-s) - \exp(s) < 0$. Note that
    \begin{gather}
        r'(s) = 2 - \exp(-s) - \exp(s) < 0,
    \end{gather}
    and $r(0+) = 0$. Therefore, $r(s)<0$.     
\end{proof}

\begin{proof}[Proof of Proposition \ref{prop:phi_gsm}]
    From Eq. \eqref{eq:pg-sigmoid}, we have 
    \begin{equation}
        \phi(x) = (2\pi)^{-1} \int_{0}^{\infty} \exp\left( - x^2 \omega /2 \right) \operatorname{PG}(\omega \mid 1, 0) \dd \omega,
    \end{equation}
    and so
    \begin{equation}
        \phi(x) = \int_{0}^{\infty} \underbrace{\omega^{1/2} (2\pi)^{-1/2} \exp\left( - x^2\omega / 2\right)}_{\mathcal{N}\left(x \mid 0, \omega^{-1}\right)} \underbrace{(2\pi\omega)^{-1/2} \operatorname{PG}(\omega \mid 1, 0)}_{\phi_{\omega}(\omega)} \dd\omega. 
    \end{equation}
    It is clear that $\phi_{\omega}(\omega) \geq 0$ for each $\omega \in \left] 0, +\infty\right[$. To show that it integrates to 1, we integrate with respect to $x$ in Eq. \eqref{eq:phi_gsm_rep} and apply the Fubini theorem
    \begin{align}
        1 & = \int_{-\infty}^{+\infty} \int_{0}^{\infty} \mathcal{N}\left(x \mid 0, \omega^{-1}\right) \phi_{\omega}(\omega) \dd \omega \dd x = \\
        & = \int_{0}^{\infty} \left\{\int_{-\infty}^{+\infty} \mathcal{N}\left(x \mid 0, \omega^{-1}\right)\dd x \right\} \phi_{\omega}(\omega) \dd \omega = \int_{0}^{\infty} \phi_{\omega}(\omega) \dd \omega.
    \end{align}
\end{proof}
